# Supplementary material for: Characterizing Hydration Properties Based on the Orientational Structure of Interfacial Water Molecules
Source: arXiv:1708.07186 source file (2017-08-23)
Supplement: Supplementary file 1 [file SI.pdf]

# Supporting Information

# 1 Ideal hydrophobic reference system

Our chosen reference system was an ideal hydrophobic surface. Following the results of Ref. 1, we thus utilized the instantaneous liquid-vapor interface as our hydrophobic reference system. Specifically, $P(\vec{\kappa}|\text{phob})$ was computed from a simulation of a slab of 4913 SPC/E water molecules [2] in a simulation cell measuring approximately $6 \times 6 \times 10\ \text{nm}^3$. At 298 K, this simulation spontaneously forms a free liquid-vapor interface, which serves to buffer the pressure of the liquid region of the slab. Figure S1 shows the value of $f(\vec{\kappa}|\text{phob})$ for several different values of a, i.e., the molecular distance from the instantaneous liquid interface.

# 2 Simulations of the patterned silica surfaces

Simulations consisted of a slab of 4913 water molecules, modeled with the SPC/E force field, in a periodically replicated cell with x, y, and z, dimensions of 5.932 nm, 5.982 nm, and 10.00 nm respectively. At the lower z boundary of the simulation cell is a model silica substrate. The details of the substrate and its interactions with SPC/E water molecules is described in Ref. 3. Simulations were carried out using LAMMPS [4] with a NVT ensemble, and $T = 298$

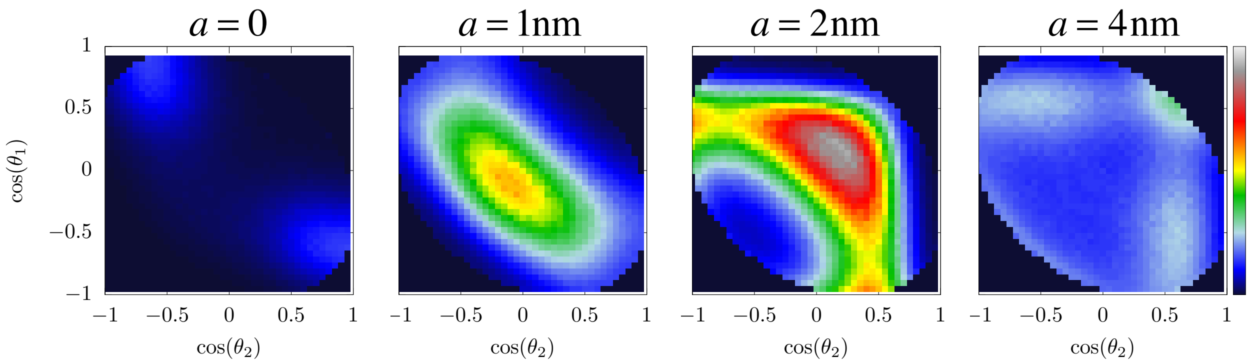


Figure S1: Figures show the value of the orientational distribution function $f(\vec{\kappa}|\text{phob})$, as indicated by shading. Each plot is scaled to the same color bar.

K, enforced via a Langevin thermostat. The volume of the liquid water slab is much less than that of the simulation cell. This results in the formation of a liquid-vapor like phase boundary that serves to effectively buffer the pressure of the liquid slab.

Surface maps of $\delta\lambda_{\mathrm{phob}}$ were generated via the following procedure. The surface was divided into a square lattice of surface points. The lattice spacing for this division is arbitrary. Following Eq. (3) in the main text we computed $\delta\lambda_{\mathrm{phob}}$ by assigning exactly one water molecule to each surface point for every output simulation snapshot (each water molecule can be assigned to multiple surface points). This ensures that $\delta\lambda_{\mathrm{phob}}$ for each surface point is averaged over an identical number of molecular configurations, $\vec{\kappa}$. In particular, we project the silhouette of each water molecule, taken to be a sphere of radius 2 Å onto the solute surface. The water molecule assigned to a given surface point is the closest molecule to the surface that has a silhouette covering the given surface point.

The color scale from the main text was selected based on the statistics of $\delta\lambda_{\mathrm{phob}}$ computed within the reference system using $\tau = 20$ ps. Figure S2 shows the probability distribution, $P(\delta\lambda_{\mathrm{phob}})$, computed within environment of the hydrophobic reference system

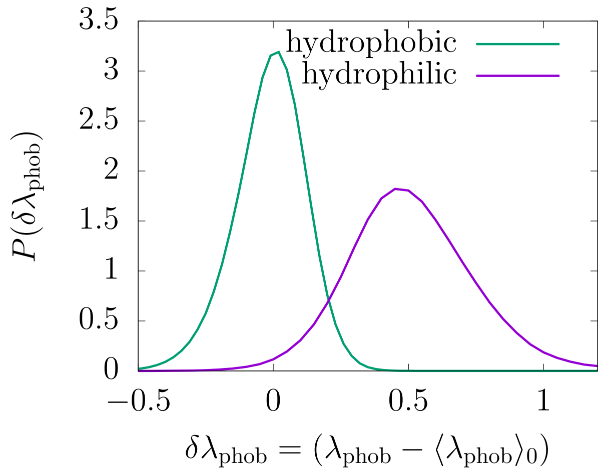


Figure S2: The probability distribution for $\delta\lambda_{\mathrm{phob}}$ computed using $\tau = 20$ ps for an ideal hydrophobic reference system ("hydrophobic") and for a fully hydroxylated model silica surface ("hydrophilic").

(labeled "hydrophobic") and the environment of a fully hydroxylated silica surface (labeled "hydrophilic"). This figure illustrates two important points: (1) the hydrophobic and hydrophilic distributions are well separate, which makes $\delta\lambda_{\mathrm{phob}}$ a good order parameter for hydrophobicity, and (2) the equilibrium fluctuations of $\delta\lambda_{\mathrm{phob}}$ for an ideal hydrophobic interface extend over a range of about $-0.3 \leq \delta\lambda_{\mathrm{phob}} \leq 0.3$. We thus interpret values of $\delta\lambda_{\mathrm{phob}} \geq 0.3$ to indicate the presence of hydrophilic surfaces.

We carried out simulations on model silica surfaces with a variety of different surface patterns. These patterns are illustrated in Fig. S3 along with corresponding maps of $\delta\lambda_{\mathrm{phob}}$ computed for $\tau = 20$ ps and $\tau = 4$ ns.

# 3 Simulations of the CheY protein

The crystal structure of inactive CheY (PDB code: 1JBE) [5] was taken for the simulation. The protein were added with hydrogen atoms and then immersed in a bath of explicit water through the AutoPSF and Solvate plugins of VMD [6]. The protein atoms are described by the all-atom CHARMM22 force field [7]. Water molecules follow the TIP3P potential [8] adapted for the CHARMM [7]. Molecular dynamics simulation was performed in an NVT ensemble using the LAMMPS package [REF.4]. There are 8059 water molecules in the simulation cell with dimensions of $6.0 \times 6.0 \times 12.0$ nm, and the system is of slab geometry. The slab is about 7 nm thick and the protein was ensured to be in the bulk liquid phase during the simulation. The system was equilibrated at $T = 298$ K, enforced via a Langevin thermostat. Particle Mesh Ewald was used to handle the long-range part of electrostatic interactions. The SHAKE algorithm was used to constrain the geometry of water.

As shown in Figure 4 of the main text, $\delta\lambda_{\mathrm{phob}}$ was computed along the protein surface with temporal resolution. For the characterization, the coordinates of protein atoms were averaged over $\tau = 10$ ps and a Willard-Chandler surface was constructed, which encloses the protein, following the procedure given in Ref. 9. In the construction, the coarse-grained density was calculated on a cubic lattice with the spacing of 1.0 Å, using the Gaussian coarse-graining length of 2.0 Å (for all atoms of protein). The half of bulk water density was used

for the criterion of locating the surface. Each surface point is assigned with the nearest water from the first hydration shell (*i.e.*, $-1\,\text{Å} < a < 3\,\text{Å}$), and $\delta\lambda_{\text{phob}}(\vec{r}_{\text{surf}}, t)$ was computed along the surface points and time frames. The corresponding reference system is the liquid-vapor interface of TIP3P water. Although its $f(\vec{\kappa}|\text{phob})$ is qualitatively similar to that of SPC/E water, the probability distribution of $\delta\lambda_{\text{phob}}$ is slightly different upon the given method of assigning water to surface points. We adapted the color scale such that we interpret values of $\delta\lambda_{\text{phob}} \geq 0.375$ to indicate the presence of hydrophilic surfaces, where 0.375 is about 1.5 standard deviation of $P(\delta\lambda_{\text{phob}})$ (Fig. S4).

For the residue-based characterization, the orientational information of water molecules can be repartitioned with respect to specific residue. Per each time step, 10 water molecules in the first hydration shell, which are the closest to specific residue, were adopted for computing $\delta\lambda_{\text{phob}}$. This analysis was applied to the surface residues that are exposed to sufficient number of water molecules. The surface residues were identified by counting the water molecules observed near individual residue and the cutoff criterion was more than 15 water molecules per time step (in average).

# References


[1] Adam P Willard and David Chandler. The molecular structure of the interface between water and a hydrophobic substrate is liquid-vapor like. *The Journal of chemical physics*, 141(18):18C519, October 2014.

[2] H J C Berendsen, J R Grigera, and T P Straatsma. The missing term in effective pair potentials. *The Journal of Physical Chemistry*, 91(24):6269–6271, November 1987.

[3] Nicolas Giovambattista, Pablo G Debenedetti, and Peter J Rossky. Hydration Behavior under Confinement by Nanoscale Surfaces with Patterned Hydrophobicity and Hydrophilicity. *The Journal of Physical Chemistry C*, 111(3):1323–1332, January 2007.

[4] Steve Plimpton. Fast Parallel Algorithms for Short-Range Molecular Dynamics. *Journal of Computational Physics*, 117(1):1–19, March 1995.

[5] M Simonovic and K Volz. A distinct meta-active conformation in the 1.1-A resolution structure of wild-type ApoCheY. *The Journal of biological chemistry*, 276(31):28637–28640, August 2001.

[6] William Humphrey, Andrew Dalke, and Klaus Schulten. Vmd: visual molecular dynamics. *Journal of molecular graphics*, 14(1):33–38, 1996.

[7] Alex D MacKerell Jr, Donald Bashford, MLDR Bellott, Roland Leslie Dunbrack Jr, Jeffrey D Evanseck, Martin J Field, Stefan Fischer, Jiali Gao, H Guo, Sookhee Ha, et al. All-atom empirical potential for molecular modeling and dynamics studies of proteins. *The journal of physical chemistry B*, 102(18):3586–3616, 1998.

[8] William L. Jorgensen, Jayaraman Chandrasekhar, Jeffry D. Madura, Roger W. Impey, and Michael L. Klein. Comparison of simple potential functions for simulating liquid water. *The Journal of Chemical Physics*, 79(2):926, 1983. ISSN 00219606. doi: 10.1063/1.445869.

[9] Adam P Willard and David Chandler. Instantaneous Liquid Interfaces. *The Journal of Physical Chemistry B*, 114(5):1954–1958, February 2010.

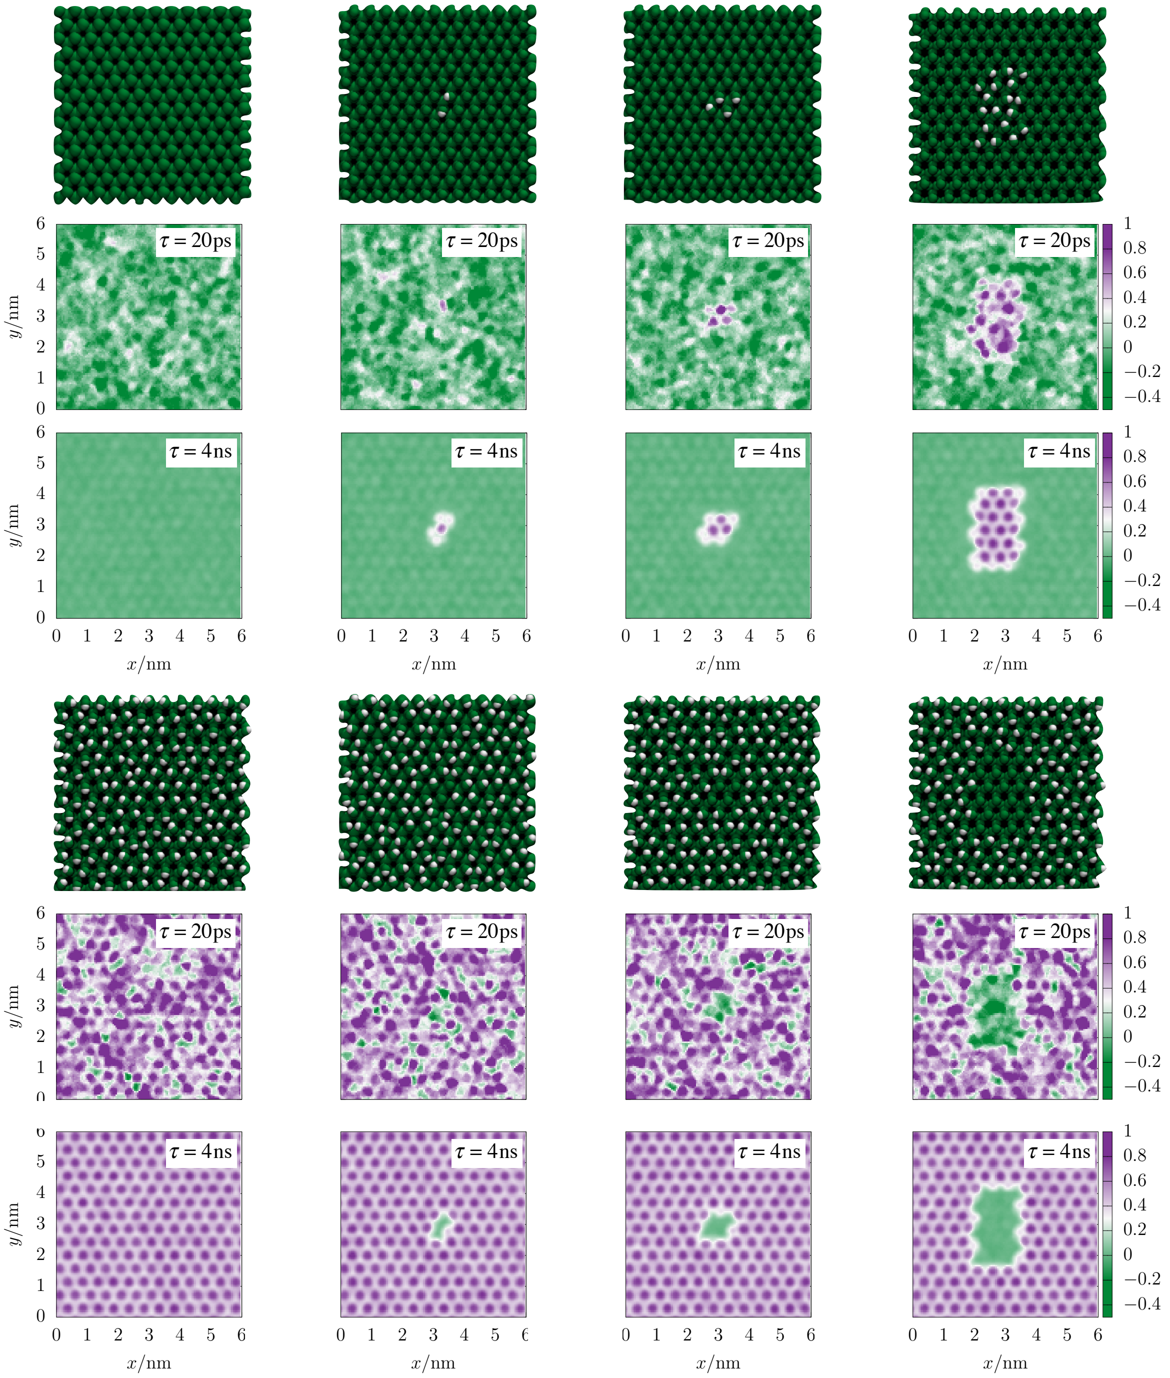


Figure S3: The interfacial structure of liquid water in contact with a series of different patterns of the model silica surface. Each different surface pattern is represented with an atomistic rendering of the model silica surface. Below each of these renderings are plot of the $\delta\lambda_{\text{phob}}$, computed according to Eq. (3) in the main text, with $\tau = 20$ ps and $\tau = 4$ ns.

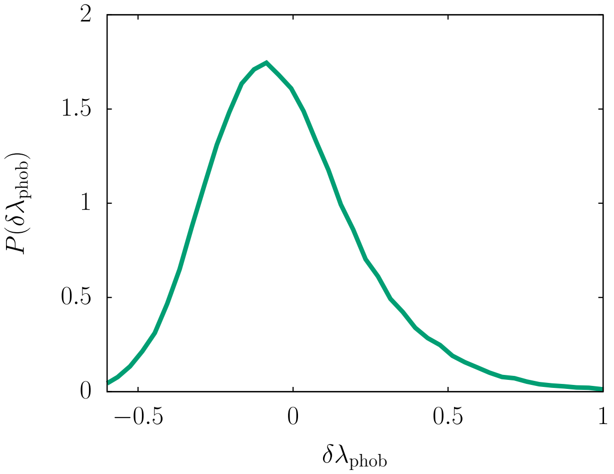


Figure S4: The probability distribution for $\delta\lambda_{\mathrm{phob}}$ computed using $\tau = 20$ ps for an ideal hydrophobic reference system ("hydrophobic") and for a fully hydroxylated model silica surface ("hydrophilic").
